# Supplementary material for: Electron Interaction Effects in Periodically Driven Kitaev Model: Topology Breaking and Enhancement of Quantum Chaos
Source: arXiv:1604.06700 source file (2016-05-10)
Supplement: Supplementary file 1 [file Appendix.pdf]

# Appendix

May 10, 2016

## 1 The effective Hamiltonian for $V = 0$

In the absence of the interaction ($V = 0$), the model reduces to the period driving Kitaev chain, in which the existence of Majorana edge modes providing that it is in the topological phase. The operators $c_j$ satisfy the usual anticommutation relations $\{c_m, c_n\} = 0$ and $\left\{c_m, c_n^\dagger\right\} = \delta_{mn}$. Introducing the Majorana operators

$$a_{2j-1} = c_j + c_j^\dagger \quad \text{and} \quad a_{2j} = -i\left(c_j - c_j^\dagger\right) \tag{1.1}$$

for $j = 1, 2, \cdots, N$, it can be checked that these are Hermitian operators satisfying $\{a_m, a_n\} = 2\delta_{mn}$. In terms of these operators, the single-particle Hamiltonian takes the form

$$h = \frac{i}{4}\sum_{m,n=1}^{2N} a_m M_{mn} a_n \tag{1.2}$$

where $M$ is a real antisymmetric matrix with $M_{2n,2n+1} = -M_{2n+1,2n} = \tilde{t} + \Delta$, $-M_{2n-1,2n+2} = M_{2n+2,2n-1} = (\tilde{t} - \Delta)$ and $-M_{2n-1,2n} = M_{2n,2n-1} = \mu$. The Hamitonian is quadratic in terms of Majorana fermions and the Floquet operator is obtained as $U_f(T, 0) = e^{M_2T/2}e^{M_1T/2}$, where $M_1$ and $M_2$ are antisymmetric matrices with parameter $\mu = \mu_0 + \delta\mu$ and $\mu = \mu_0 - \delta\mu$, respectively. The spectrum of $U_f(T, 0)$ are given by phase of $e^{i\theta_j T}$ and they come from the complex conjugate pairs reflecting the particle-hole symmetry, $U_f(T, 0)\psi_j = e^{-i\theta_j T}\psi_j$ implying $U_f(T, 0)\psi_j^* = e^{i\theta_j T}\psi_j^*$.

By applying the linear transformation,

$$\vec{f} = \mathbf{B}\vec{a}, \tag{1.3}$$

$U_f(T, 0)$ transforms to $U_f = e^{-ih_f T}$, with the effect Hamiltonian $h_f = \sum_{j=1}^{L}\theta_j(f_j^\dagger f_j - \frac{1}{2})$ and $0 \le \theta_j \le \pi$. Here $\vec{f} = (f_1, f_1^\dagger, \cdots f_N, f_N^\dagger)$ and $\vec{a} = a_1, a_2, \cdots, a_{2N}$. $\mathbf{B}$ is a (2N)-dimensional matrix with the $(2j-1)$th ($2j$th) row being $\psi_j^*$ ( $\psi_j$), where $\psi_j$ the eigenvector of $U_f(T, 0)$ with eigenvalue $e^{-i\theta_j T}$. $f_j$ and $f_j^\dagger$ are Dirac fermion operators. We also arrange the single-particle quasienergies $\theta_j$ in an increasing order such that $f_1$ ($f_1^\dagger$) is the annihilation (creation) operator for the zero mode.

## 2 Physical meaning of $\tilde{N}_1 - \tilde{N}_0$ for $V = 0$

To show that $\tilde{N}_1 - \tilde{N}_0$ actually reflects the fading of Majorana zero mode during the topological phase transition, we first consider $V = 0$ by quenching $\mu_0$. In the Heisenberg picture

$$\tilde{N}_1 - \tilde{N}_0 = \left\langle 0 \left| f_1 f_1^\dagger(t) f_1(t) f_1^\dagger \right| 0 \right\rangle - \left\langle 0 \left| f_1^\dagger(t) f_1(t) \right| 0 \right\rangle. \tag{2.1}$$

Since $h_f(t)$ is quadratic, $\vec{f}(t) = \mathbf{B}\vec{a}(t) = \vec{B}S(T, 0)\vec{a}$, with $S(t, 0) = \mathcal{T}\exp\int_0^t M(t')\mathrm{d}t'$ the time evolution operator. Therefore the relation between $\vec{f}(t)$ and $\vec{f}$ is given by

$$\vec{f}(t) = \mathbf{B}S(t, 0)\mathbf{B}^{-1}\vec{f} \equiv \mathbf{S}\vec{f}. \tag{2.2}$$

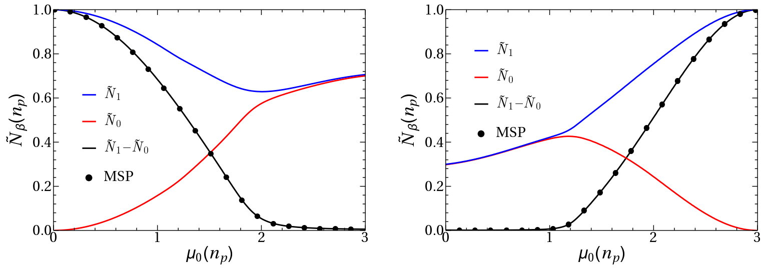


(a) (b)

Figure 1: Majorana survival probability (MSP) and $\tilde{N}_\beta$ for the zero mode (a) and the $\pi$ mode (b), respectively. In (a) (or (b)) the system is initiated at $\mu_0 = 0$ (or $\mu_0 = 3.0$), and slowly changes to $\mu_0 = 3.0$ (or $\mu_0 = 0.0$) with $N_T = 2000$ time period. The other parameters are set to $V = 0$, $L = 20$, $\delta\mu = 2.5$ and $T = 1$.

Substituting Eq. 2.2 into Eq. 2.1, it can be shown that

$$\begin{aligned} N_1 - N_0 &= \mathbf{S}_{1,1}\mathbf{S}_{2,2} - \mathbf{S}_{2,1}\mathbf{S}_{1,2} \\ &= \left|\langle\psi_1\left|S(t,0)\right|\psi_1\rangle\right|^2 - \left|\langle\psi_1\left|S(t,0)\right|\psi_2\rangle\right|^2 \qquad (2.3) \\ &\approx \left|\langle\psi_1|\psi_1(t)\rangle\right|^2. \qquad (2.4) \end{aligned}$$

Here $\psi_1(t)$ is the time evolution of $\psi_1$ at $t$ after quenching. In the last equation we use the fact that for a sufficient long chain, the two wave functions with zero quasienergy can always be expressed as $\psi_1 = \phi_L + i\phi_R$ and $\psi_1 = \phi_L - i\phi_R$, with $\phi_L$ ($\phi_R$) being real and localized at the left(right) end. $\left|\langle\psi_1\left|S(t,0)\right|\psi_2\rangle\right|^2 \approx 0$. From Eq. 2.2 we can see that $\tilde{N}_1 - \tilde{N}_0$ is nothing but the Majorana survival probability(MSP) after quenching. The comparison of MSP with $\tilde{N}_1 - \tilde{N}_0$ for the zero mode and $\pi$ mode are illuminated in Fig. 1(a) and Fig. 1(b), respectively.
